# Supplementary material for: U-TELL: Unsupervised Task Expert Lifelong Learning
Source: arXiv:2405.14623 source file (2024-06-10)
Supplement: Supplementary file 1 [file X_suppl.tex]

\clearpage
\setcounter{page}{1}
% \maketitlesupplementary
\maketitle 
% \section{Rationale}
% \label{sec:rationale}
% % 
% Having the supplementary compiled together with the main paper means that:
% % 
% \begin{itemize}
% \item The supplementary can back-reference sections of the main paper, for example, we can refer to Section \ref{sec:intro};
% \item The main paper can forward reference sub-sections within the supplementary explicitly (e.g. referring to a particular experiment); 
% \item When submitted to arXiv, the supplementary will already included at the end of the paper.
% \end{itemize}
% % 
% To split the supplementary pages from the main paper, you can use \href{https://support.apple.com/en-ca/guide/preview/prvw11793/mac#:~:text=Delete%20a%20page%20from%20a,or%20choose%20Edit%20%3E%20Delete).}{Preview (on macOS)}, \href{https://www.adobe.com/acrobat/how-to/delete-pages-from-pdf.html#:~:text=Choose%20%E2%80%9CTools%E2%80%9D%20%3E%20%E2%80%9COrganize,or%20pages%20from%20the%20file.}{Adobe Acrobat} (on all OSs), as well as \href{https://superuser.com/questions/517986/is-it-possible-to-delete-some-pages-of-a-pdf-document}{command line tools}.
% Supplementary 
\section{Datasets}
\label{AppendixA}
The wafer defect map dataset is collected \cite{wang2020deformable} from the semiconductor wafer manufacturing industry. 
We select ten classes for conducting the Class-IL experiment with training and testing sets of 1700 and 200 samples per task respectively. First, we conduct the Class-IL experiments for SMNIST, SCIFAR10, and SSVHN with a training set of 10000 samples per task and a test set of 1000 samples per task. 
We implement the Class-IL setting with SMNIST, SCIFAR10, SSVHN, STinyImagenet, SWAFER datasets with five tasks $(t_1, t_2, t_3, t_4, t_5)$ where each task has two mutually exclusive classes $(\{\{0,1\}, \{2,3\}, \{4,5\}, \{6,7\}, \{8,9\}\})$. CIFAR100 datastream has a sequence of 10 tasks ($t_1,\ldots,t_{10}$) with a total of 20 coarse classes and 2 classes per each task \cite{yu2023scale}. Next, we carry out Domain-IL setting with RMNIST and PMNIST datasets with four task sequences $(t_1, t_2, t_3, t_4$).
% with a training set of 15000 samples per task and a test set of 1250 samples per task.
We construct the PMNIST dataset by giving a distribution drift through random permutations to the original MNIST dataset. We create the RMNIST dataset by random rotations of $\{[0-30],[31-60], [61-90], [91-120]\}$ degrees to the original MNIST dataset corresponding to four tasks following the experiment settings of \cite{pratama2021unsupervised}. 
Class-IL split datastream introduces two classes per task. We generate the Class-IL stream for SMNIST, SCIFAR10, and SSVHN by randomly selecting 5000 samples for each of the selected two classes per task. Randomly selected 500 non-overlapping samples per class are used to create the test dataset for SMNIST, SCIFAR and SSVHN. Wafer defect data contains normal, single defect and multi-defect data with ten classes. SWAFER train datastream for each task has two classes and contains 950 randomly selected samples per class and the test dataset contains 50 samples per class. The SMNIST, SCIFAR10, SSVHN, SWAFER datastreams contain five sequential tasks $(t_1,t_2,t_3,t_4,t_5)$ with two mutually exclusive classes per task, $\{\{0,1\},\{2,3\},\{4,5\},\{6,7\},\{8,9\}\}$. Domain-IL training datastreams of RMNIST and PMNIST contain 10 classes per task, 1500 randomly selected samples per class and a total of 15000 samples per task. Test data contains 125 randomly selected non-overlapping data per class. 
% In Class-IL setting, all models are trained with fiv

Domain-IL datastream has four tasks, $(t_1,t_2,t_3,t_4)$. RMNIST datastream is created by giving random rotations of $\{[0-30], [31-60], [61-90], [91-120]\}$ for tasks $t_1$ to $t_4$ respectively, to the original MNIST data. PMNIST task sequence $t_1$ to $t_4$ is generated by giving random permutations to the original MNIST image pixels.  

Please note that we use similar settings for the training of all selected baselines. Train and test datastreams are generated by invoking functions of publicly available utilsADCN.py from \href{url}{https://tinyurl.com/AutonomousDCN}.  
\section{Training process details}
\label{AppendixB}
Let us consider the Class-IL training, e.g., SMNIST dataset, at $0^{th}$ instant $\tau = 0$, we receive the first task $t_1$ with two disjoint classes $\{0,1\}$. Now we introduce the first task expert $TE_1$. As explained in section \ref{sec:method}, each $TE$ block has three modules; an encoder-decoder module, a $k$-means clustering module and a task structure signature extractor. Further, we continue to receive the remaining sequence of tasks, $t_2,\ldots,t_k$ and accordingly we train $TE$s for each task. After $TE_k$ is ready, the $SDG$ block performs the generation of structured samples with the help of stored task structure signatures. Now, we train the $TA$ to direct the test samples to $TE$s. This completes the training process of Class-IL datastream.

Now let us discuss the Domain-IL training, e.g., RMNIST datastream. Initially at $\tau = 0$, we receive the first task $t_1$ and it has ten classes. We introduce $TE_1$ to learn $t_1$ task distribution and we continue dynamically adding more $TE$s as we keep receiving $t_2,\ldots,t_k$. During the testing phase, we generate structured samples in $SDG$ for all $t_1,\ldots,t_k$ tasks and perform a similarity check with test samples to identify the task and pass on the samples to a matching $TE$.

Let us consider the case of reception of yet another task $t_{k+1}$ after the training completion of UExL. In Class-IL, we can handle the task $t_{k+1}$ by adding a new $TE_{k+1}$, followed by the generation of structured samples and re-training of $TA$. In Domain-IL, $TE_{k+1}$ is introduced to learn the $t_{k+1}$ task distribution and during the testing phase, the test samples are matched with all task structured samples to find the matching $TE$. 
\section{Additional Experiments}
\label{AppendixC}

% \begin{table}[!h]
% \centering
% \fontsize{7}{9}\selectfont
% \setlength{\tabcolsep}{3pt}
% \captionsetup{font=footnotesize}
% \caption{Performance comparison of UExL with selected baselines on CIFAR100 and TinyImageNet }
% \begin{tabular}{ccc}
% \hline
% \multirow{2}{*}{Method} & \multicolumn{2}{c}{\textbf{Dataset}}  \\ \cmidrule{2-3} & \multicolumn{1}{c}{SCIFAR100} & \multicolumn{1}{c}{STinyImageNet}  \\
% \hline
% SCALE &13.68$\pm$0.78 &21.66$\pm$0.68 \\
% CaSSLe &10.97$\pm$0.84 &20.66$\pm$1.35 \\
% UPL-STAM &13.13$\pm$0.46 &21.68$\pm$1.30 \\
% \textbf{UExL} &\textbf{16.79$\pm$0.38} &\textbf{27.78$\pm$1.13} \\
% \hline
% \end{tabular}
% \label{tab:add_exps} 
% \end{table}
We run the evaluation of our proposed UExL method on larger datasets such as CIFAR100 \cite{krizhevsky2014cifar} and a subset of TinyImageNet \cite{deng2009imagenet} for further analysis of its performance. CIFAR100 datastream has a sequence of 10 tasks ($t_1,\ldots,t_{10}$) with a total of 20 coarse classes and 2 classes per each task \cite{yu2023scale}. CIFAR100 train data contains 5000 training images per task and 200 non-overlapping test images per task. The subset of TinyImageNet data used in our experiments has 5 tasks ($t_1,\ldots,t_5$) with 2 classes per task \cite{yu2023scale}. TinyImageNet train data has 1000 samples per task and 100 non-overlapping test samples per task.
\begin{table}[!h]
\centering
\fontsize{7}{9}\selectfont
\setlength{\tabcolsep}{3pt}
\captionsetup{font=footnotesize}
\caption{Performance comparison of UExL with selected baselines on CIFAR100 and TinyImageNet}
\begin{tabular}{cccccc}
\hline
\multirow{2}{*}{\textbf{Dataset}} & \multicolumn{4}{c}{\textbf{Method}}  \\ \cmidrule{2-6} & \multicolumn{1}{c}{SCALE} & \multicolumn{1}{c}{CaSSLe}  
&\multicolumn{1}{c}{UPL-STAM} & \multicolumn{1}{c}{UExL} & \\
\hline
SCIFAR100 &13.68$\pm$0.78 &10.97$\pm$0.84   &13.22$\pm$0.32 &\textbf{16.79$\pm$0.38}  \\
STinyImageNet &21.66$\pm$0.68 &20.66$\pm$1.35  &21.68$\pm$1.30 &\textbf{27.78$\pm$1.13} \\
\hline
\end{tabular}
\label{tab:addl_exp} 
\end{table}

\begin{figure}[!ht]
\centering
\fontsize{7}{9}\selectfont
\includegraphics[width=0.5\textwidth]{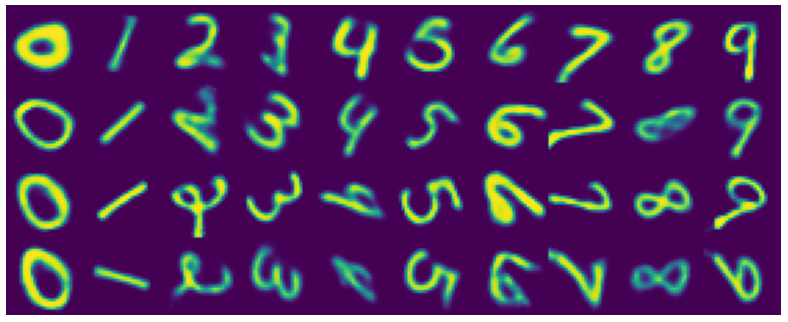} % Reduce the figure size so that it is slightly narrower than the column.
\captionsetup{font=footnotesize}
\caption{RMNIST images generated from task structure signatures}
\label{Fig3_rm_img}
\end{figure}

\begin{figure*}[ht]
\centering
\fontsize{7}{9}\selectfont
\begin{subfigure}[b]{.24\linewidth}
\fontsize{7}{9}\selectfont
\includegraphics[width=\textwidth]{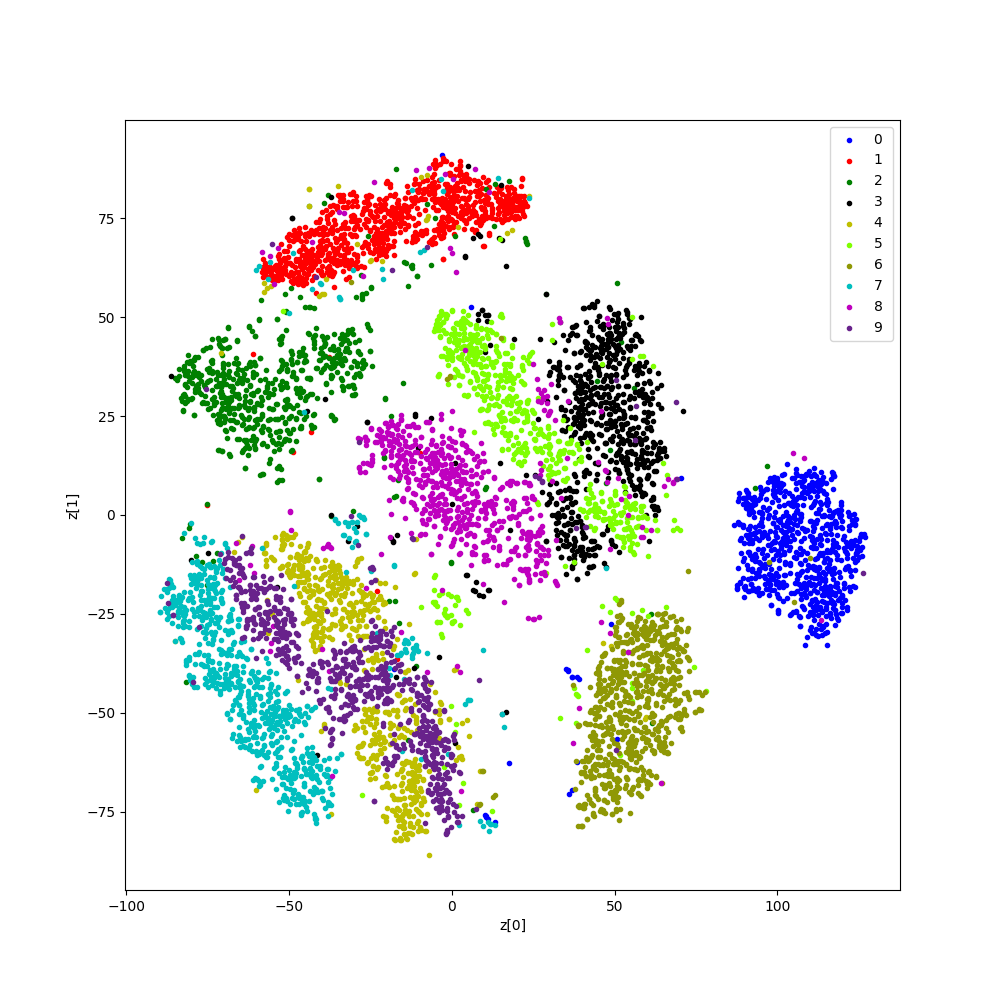} % Reduce the figure size so that it is slightly narrower than the column.
\captionsetup{font=footnotesize}
\caption{} 
\label{fig:rm_tsk1}
\end{subfigure}
\hspace{0.4cm}
\begin{subfigure}[b]{.24\linewidth}
\fontsize{7}{9}\selectfont
    \centering
\includegraphics[width=\textwidth]{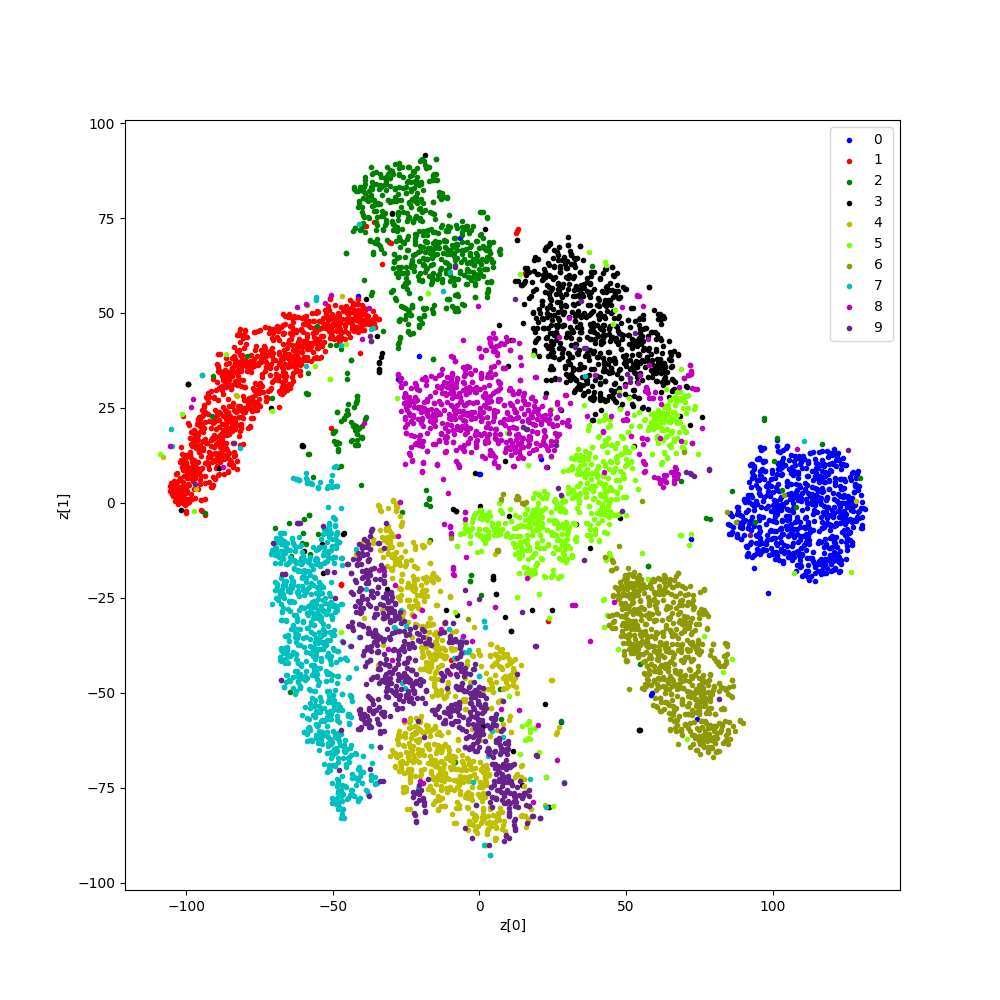} % Reduce the figure size so that it is slightly narrower than the column.
\captionsetup{font=footnotesize}
\caption{}
\label{fig:rm_tsk2}
\end{subfigure}
\begin{subfigure}[b]{.24\linewidth}
    \centering
\fontsize{7}{9}\selectfont
\includegraphics[width=\textwidth]{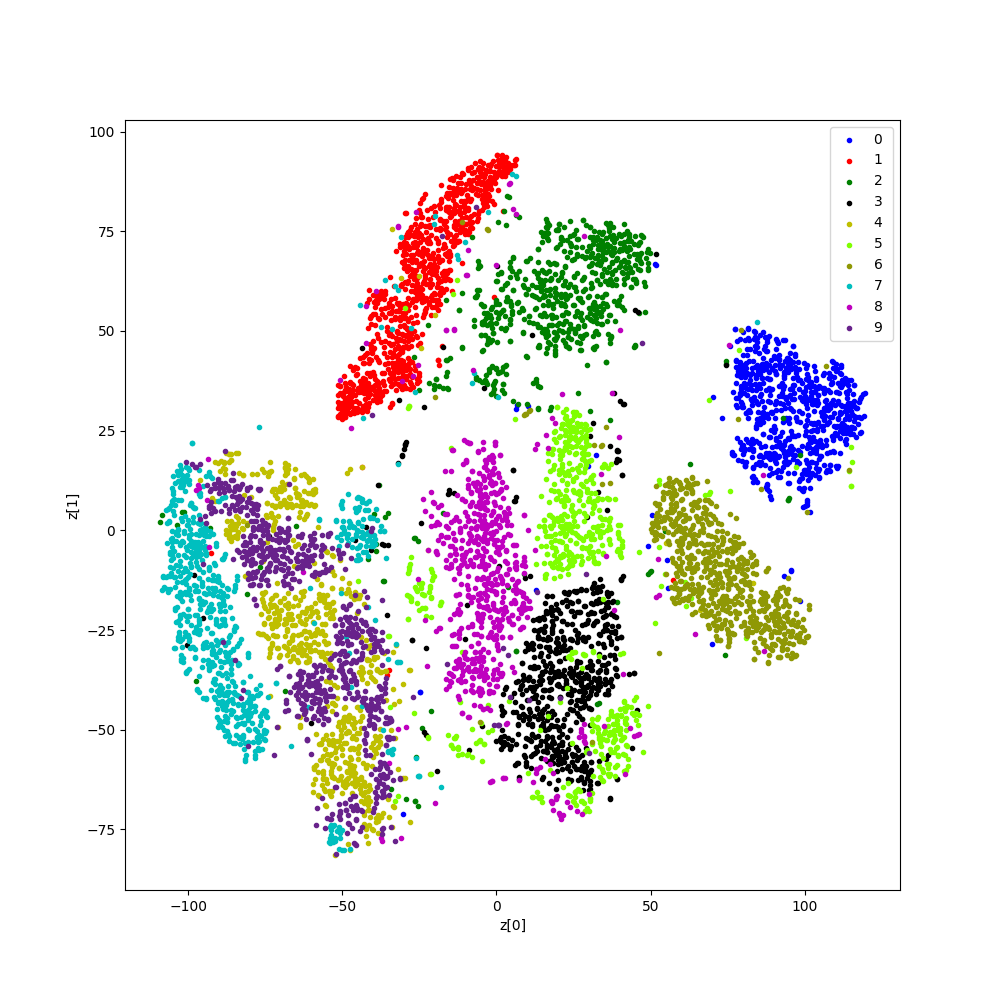} % Reduce the figure size so that it is slightly narrower than the column.
\captionsetup{font=footnotesize}
\caption{}
\label{fig:rm_tsk3}
\end{subfigure}
\begin{subfigure}[b]{.24\linewidth}
\fontsize{7}{9}\selectfont
\includegraphics[width=\textwidth]{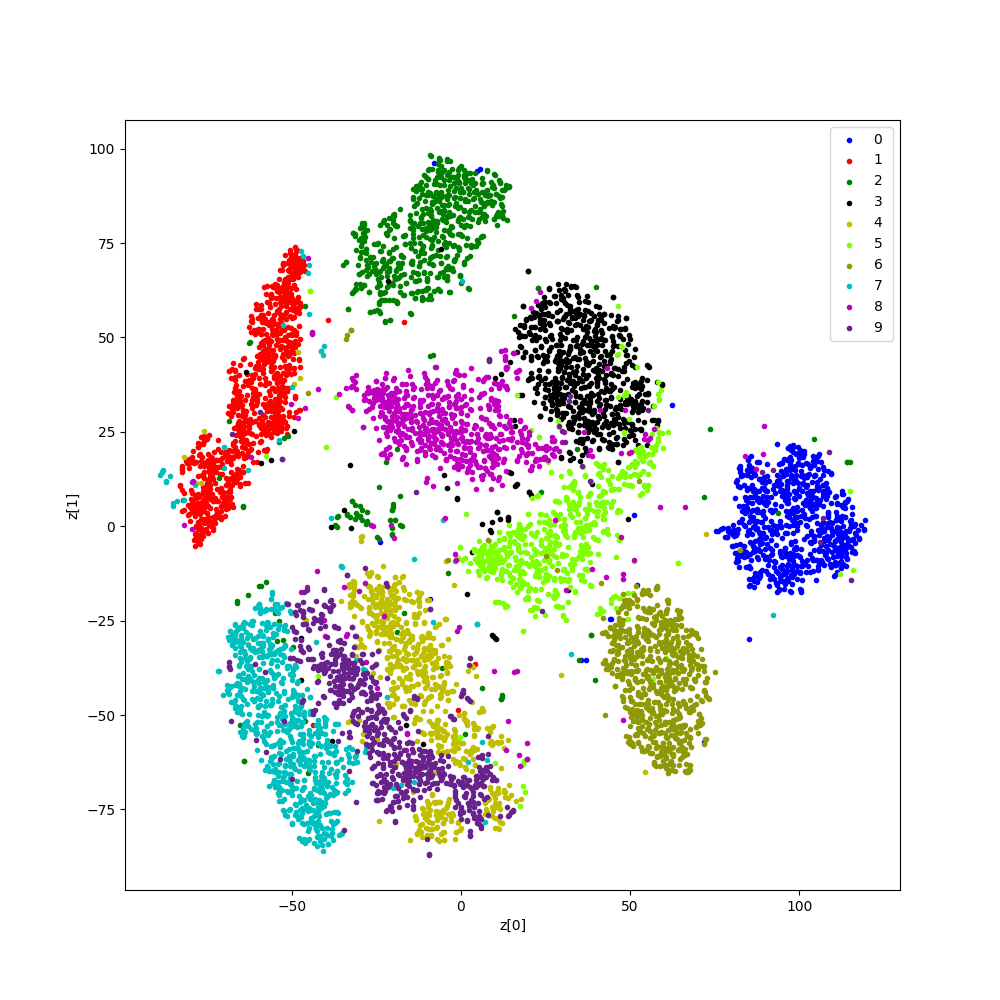} % Reduce the figure size so that it is slightly narrower than the column.
\captionsetup{font=footnotesize}
\caption{} 
\label{fig:rm_tsk4}
\end{subfigure}
\begin{subfigure}[b]{.24\linewidth}
\fontsize{7}{9}\selectfont
\includegraphics[width=\textwidth]{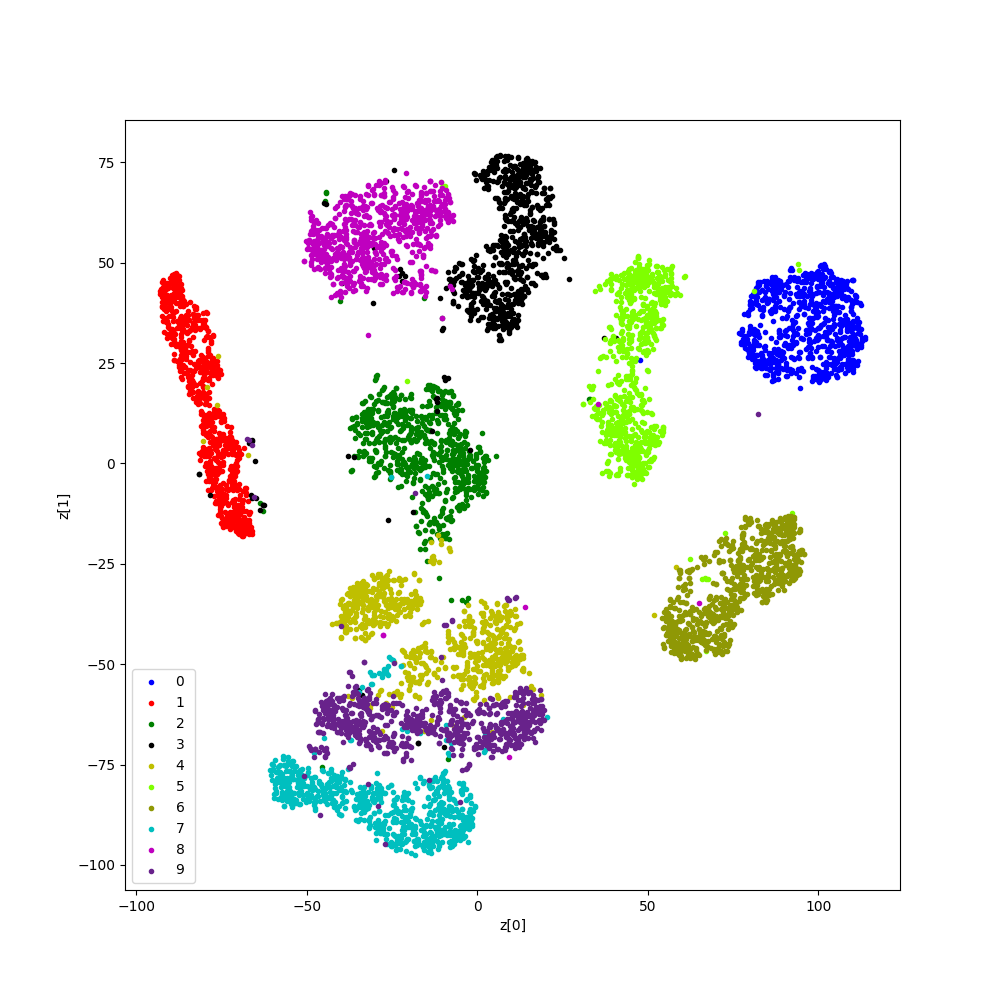} % Reduce the figure size so that it is slightly narrower than the column.
\captionsetup{font=footnotesize}
\caption{} 
\label{fig:rm_str_tsk1}
\end{subfigure}
\begin{subfigure}[b]{.24\linewidth}
\fontsize{7}{9}\selectfont
\includegraphics[width=\textwidth]{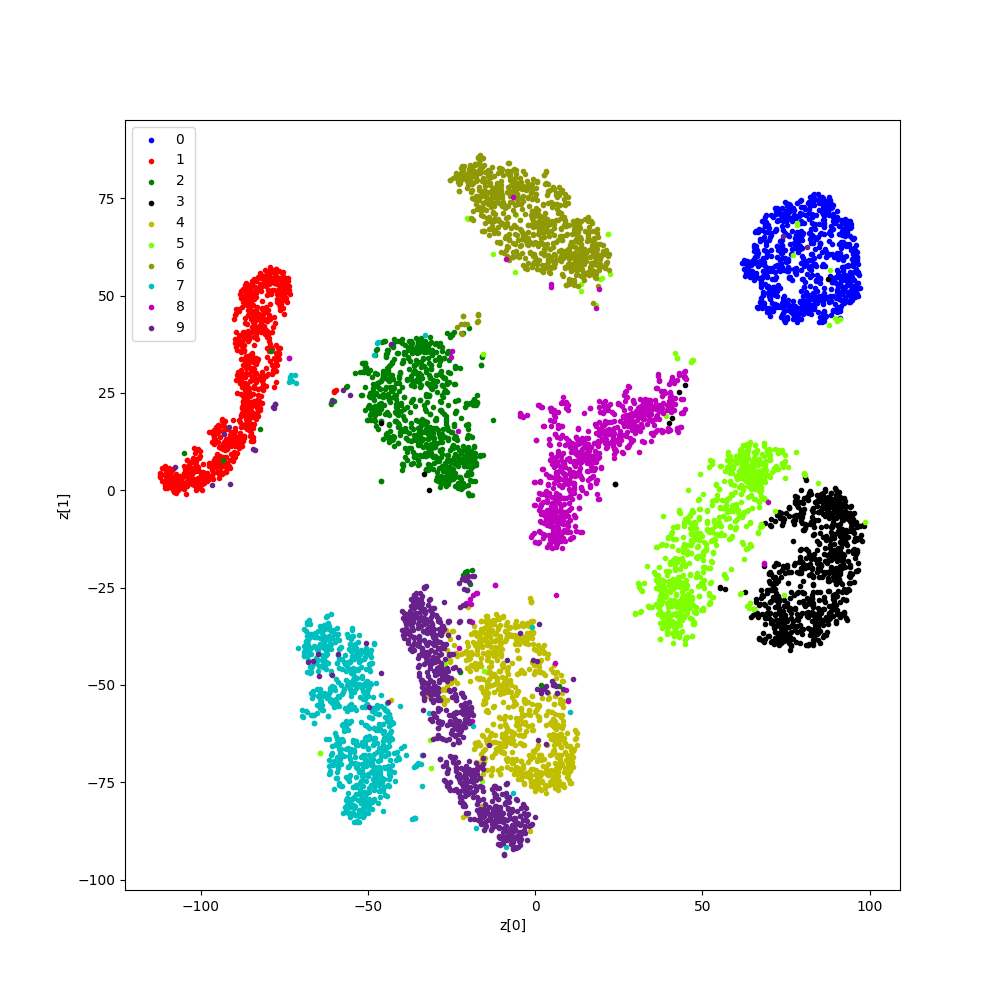} % Reduce the figure size so that it is slightly narrower than the column.
\captionsetup{font=footnotesize}
\caption{} 
\label{fig:rm_str_tsk2}
\end{subfigure}
\begin{subfigure}[b]{.24\linewidth}
\fontsize{7}{9}\selectfont
\includegraphics[width=\textwidth]{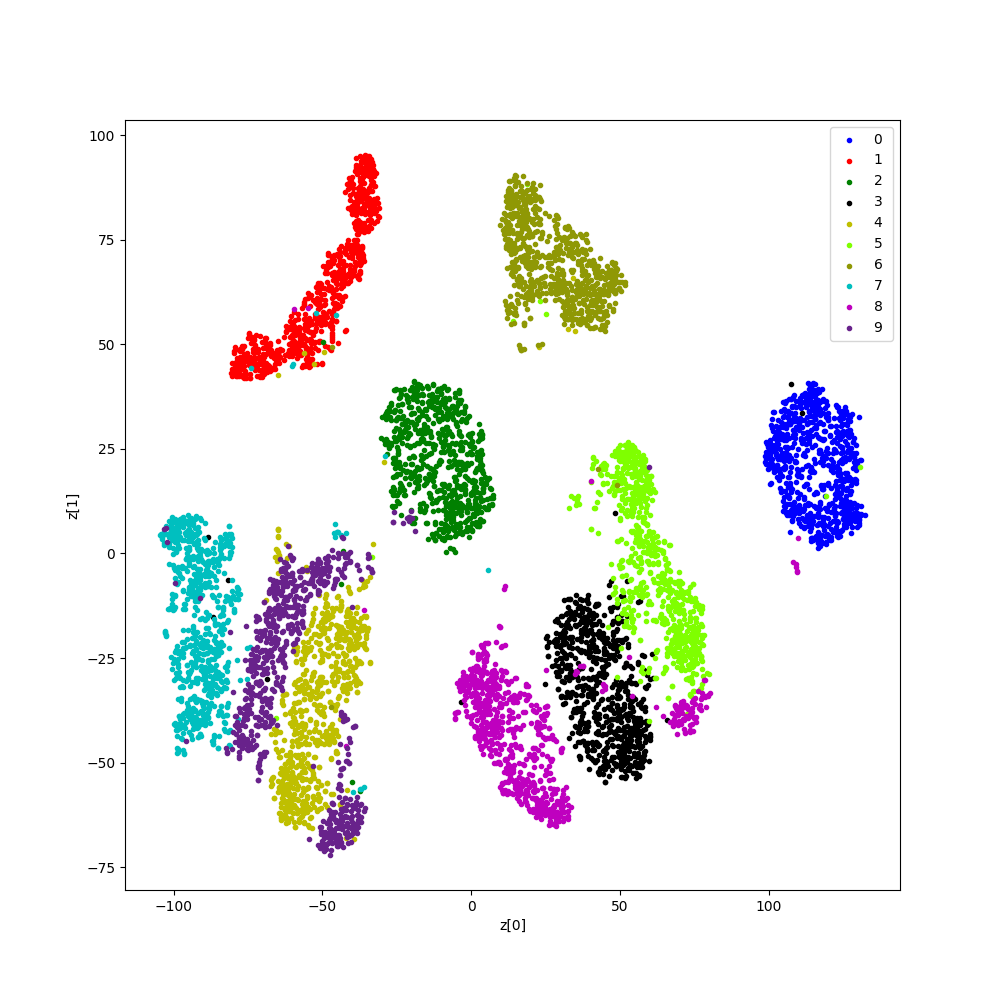} % Reduce the figure size so that it is slightly narrower than the column.
\captionsetup{font=footnotesize}
\caption{} 
\label{fig:rm_str_tsk3}
\end{subfigure}
\begin{subfigure}[b]{.24\linewidth}
\fontsize{7}{9}\selectfont
\includegraphics[width=\textwidth]{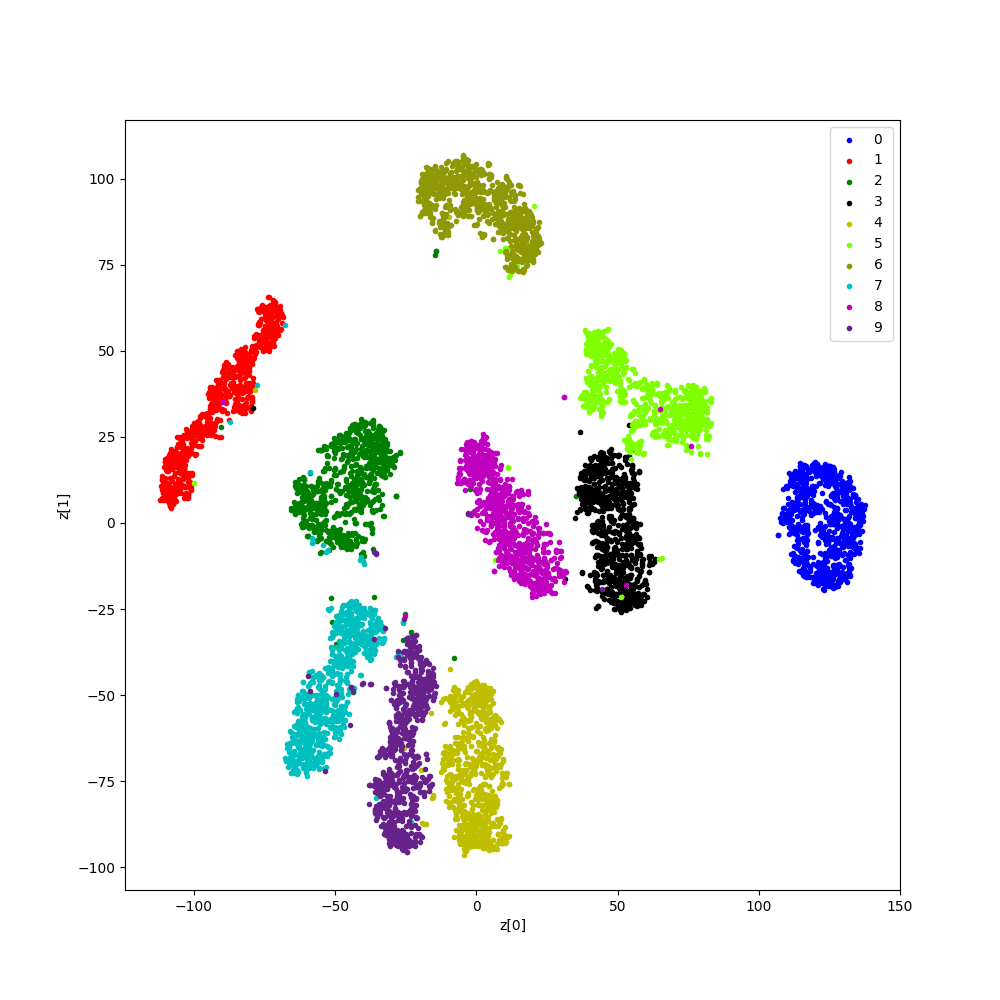} % Reduce the figure size so that it is slightly narrower than the column.
\captionsetup{font=footnotesize}
\caption{} 
\label{fig:rm_str_tsk4}
\end{subfigure}
\captionsetup{font=footnotesize}
\caption{(a)-(d) t-SNE plot of original task data $t_1$ to $t_4$ distribution, (e)-(f) t-SNE plot of generated task data $t_1$ to $t_4$ distribution.} 
\end{figure*}
Figure \ref{Fig3_rm_img} presents the Domain-IL case, displaying the RMNIST images generated by $SDG$ block (refer section \ref{sec:method}) from the stored task structure signatures. The first to fourth rows in this figure belong to generated images of task sequence $t_1$ to $t_4$. These images ascertain that the task distributions are preserved and these generated images are of good quality and are comparable to the original. Figures \ref{fig:rm_tsk1} to \ref{fig:rm_tsk4} present the t-SNE plots of original task data distribution of tasks $t_1$ to $t_4$ of RMNIST data and figures \ref{fig:rm_str_tsk1} to \ref{fig:rm_str_tsk4} are the t-SNE plots of data generated by $SDG$ block. In this case, each task has ten classes and t-SNE plots of generated data show that the task signatures are able to capture the task distributions well separated.

\begin{figure}[!ht]
\centering
\fontsize{7}{9}\selectfont
\includegraphics[width=0.5\textwidth]{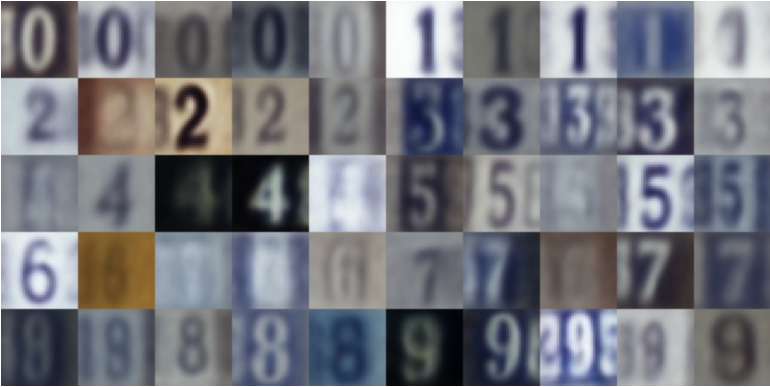} % Reduce the figure size so that it is slightly narrower than the column.
\captionsetup{font=footnotesize}
\caption{SVHN images generated from task structure signatures}
\label{Fig6_svhn_img}
\end{figure}

Figure \ref{Fig6_svhn_img} presents the $SDG$ generated images of Class-IL SSVHN tasks $t_1$ to $t_5$. Individual rows from first to fifth show the $SDG$ generated images of tasks $t_1$ to $t_5$. Figures \ref{fig:sv_tsk1} to \ref{fig:sv_tsk5} present the original task data distribution of SSVHN tasks $t_1$ to $t_5$. Here, each task has two mutually exclusive classes. Figure \ref{fig:sv_str_tsk1} to \ref{fig:sv_str_tsk5} display t-SNE plots of $SDG$ generated task samples of $t_1$ to $t_5$.

\begin{figure*}[t]
\centering
\fontsize{7}{9}\selectfont
\begin{subfigure}[b]{.18\linewidth}
\fontsize{7}{9}\selectfont
\includegraphics[width=\textwidth]{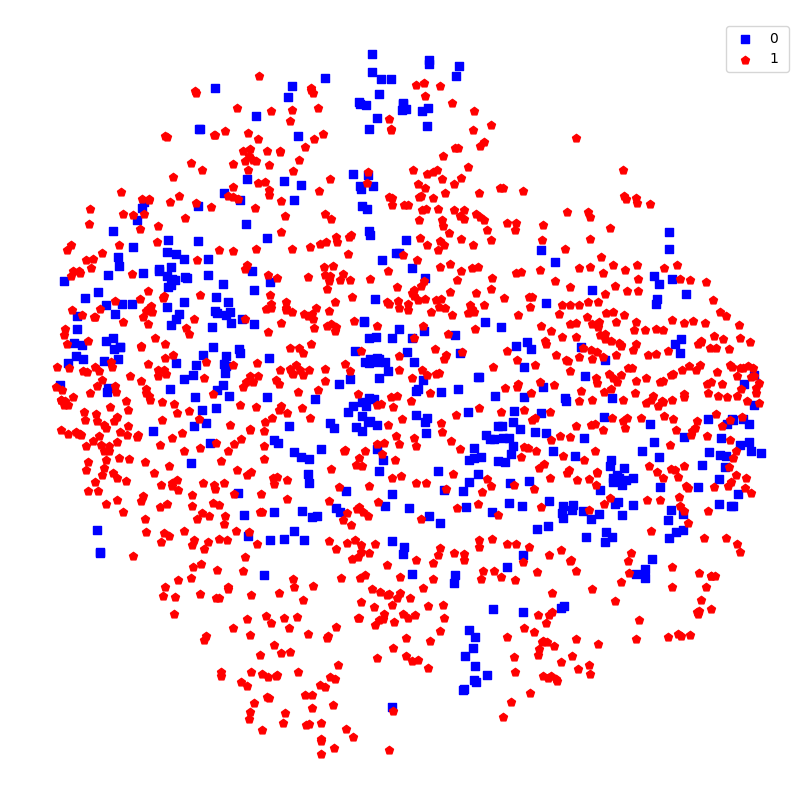} % Reduce the figure size so that it is slightly narrower than the column.
\captionsetup{font=footnotesize}
\caption{} 
\label{fig:sv_tsk1}
\end{subfigure}
\begin{subfigure}[b]{.18\linewidth}
\fontsize{7}{9}\selectfont
    \centering
\includegraphics[width=\textwidth]{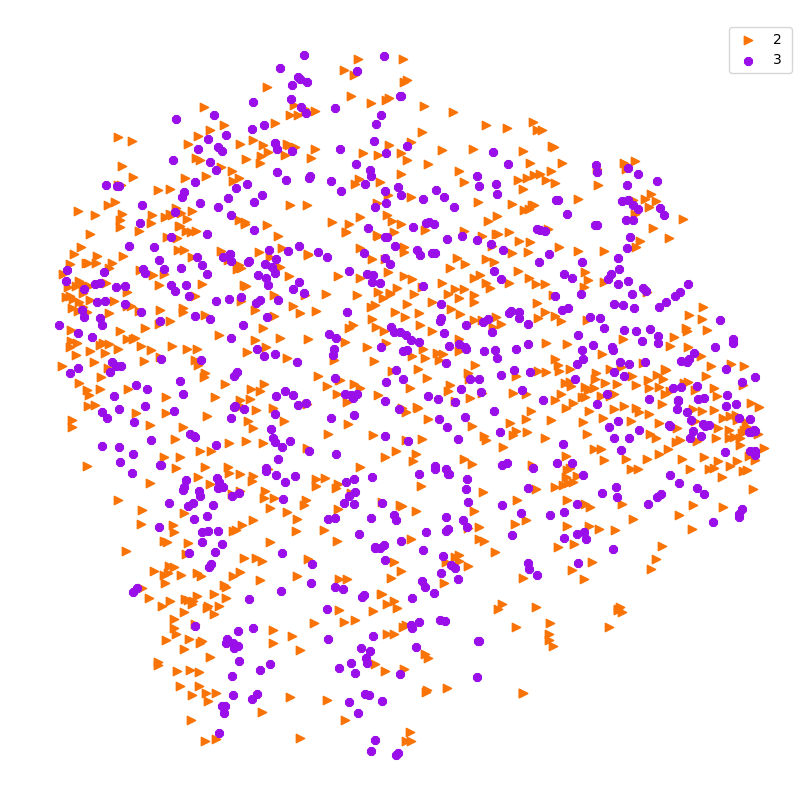} % Reduce the figure size so that it is slightly narrower than the column.
\captionsetup{font=footnotesize}
\caption{}
\label{fig:sv_tsk2}
\end{subfigure}
\begin{subfigure}[b]{.18\linewidth}
    \centering
\fontsize{7}{9}\selectfont
\includegraphics[width=\textwidth]{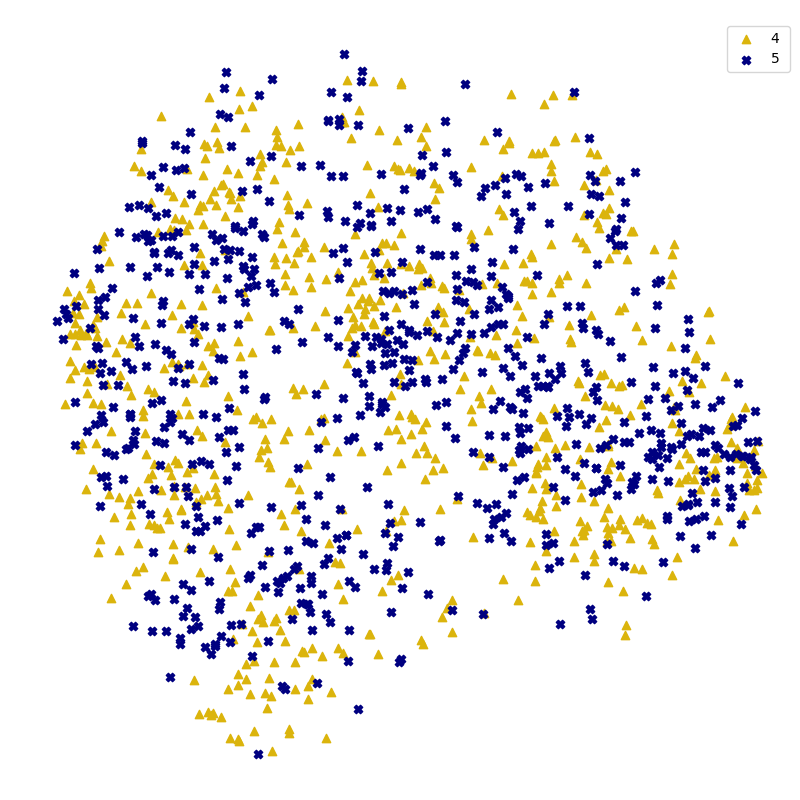} % Reduce the figure size so that it is slightly narrower than the column.
\captionsetup{font=footnotesize}
\caption{}
\label{fig:sv_tsk3}
\end{subfigure}
\begin{subfigure}[b]{.18\linewidth}
\fontsize{7}{9}\selectfont
\includegraphics[width=\textwidth]{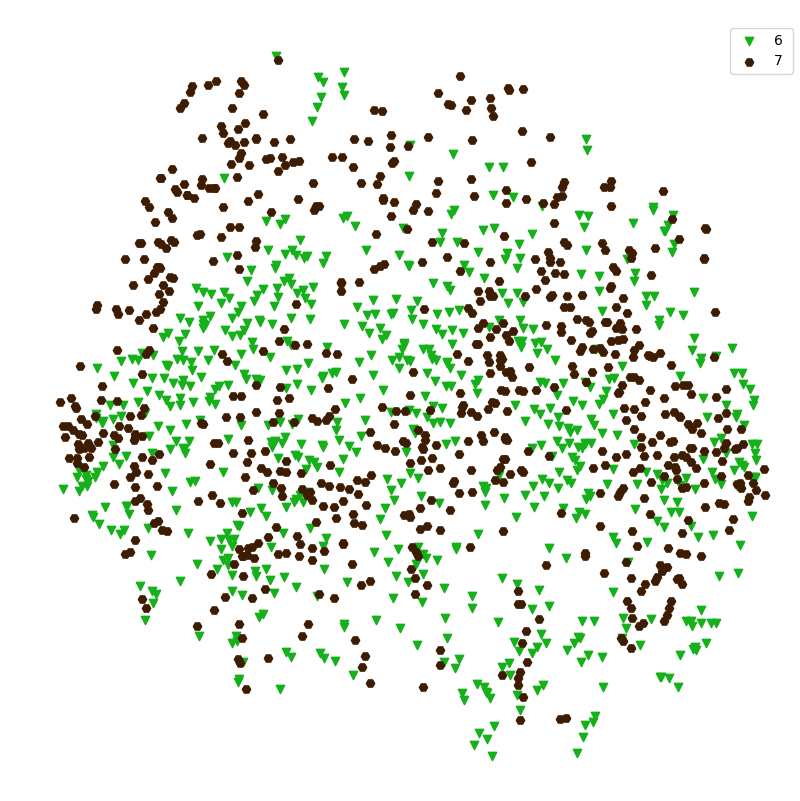} % Reduce the figure size so that it is slightly narrower than the column.
\captionsetup{font=footnotesize}
\caption{} 
\label{fig:sv_tsk4}
\end{subfigure}
\begin{subfigure}[b]{.18\linewidth}
\fontsize{7}{9}\selectfont
\includegraphics[width=\textwidth]{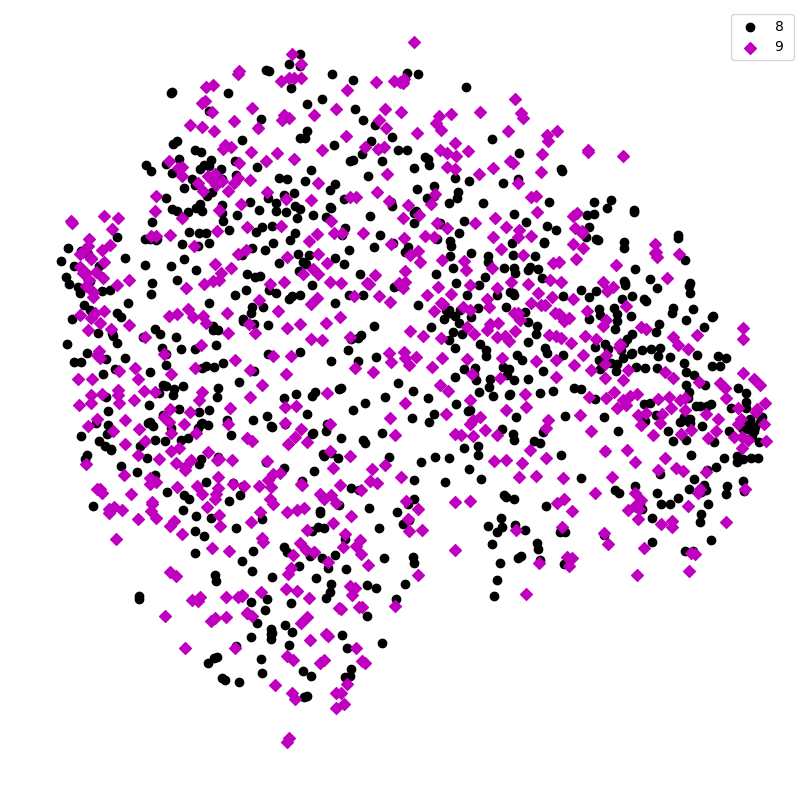} % Reduce the figure size so that it is slightly narrower than the column.
\captionsetup{font=footnotesize}
\caption{} 
\label{fig:sv_tsk5}
\end{subfigure}

\begin{subfigure}[b]{.18\linewidth}
\fontsize{7}{9}\selectfont
\includegraphics[width=\textwidth]{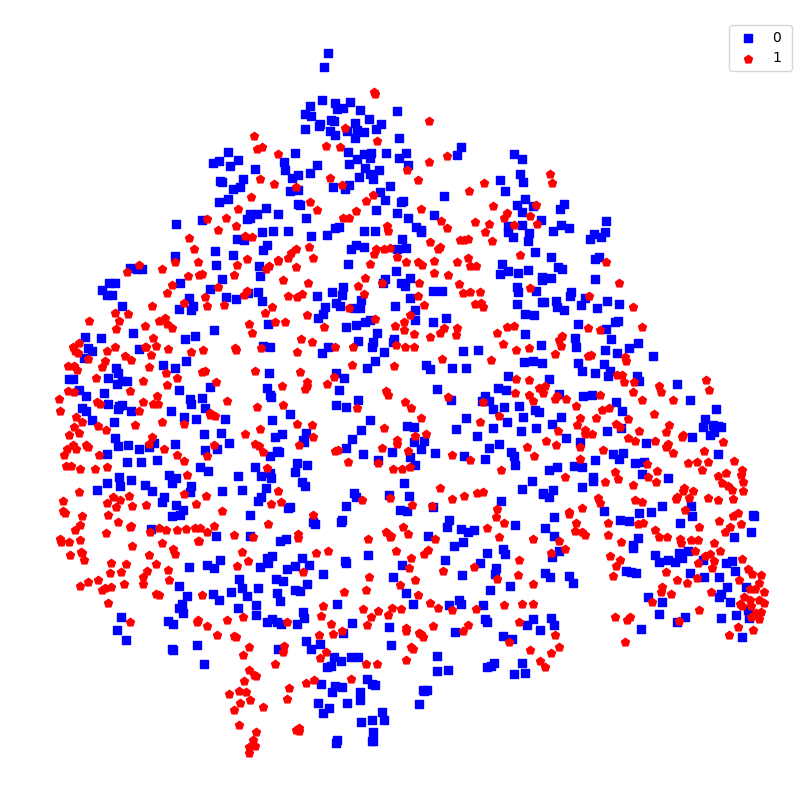} % Reduce the figure size so that it is slightly narrower than the column.
\captionsetup{font=footnotesize}
\caption{} 
\label{fig:sv_str_tsk1}
\end{subfigure}
\begin{subfigure}[b]{.18\linewidth}
\fontsize{7}{9}\selectfont
\includegraphics[width=\textwidth]{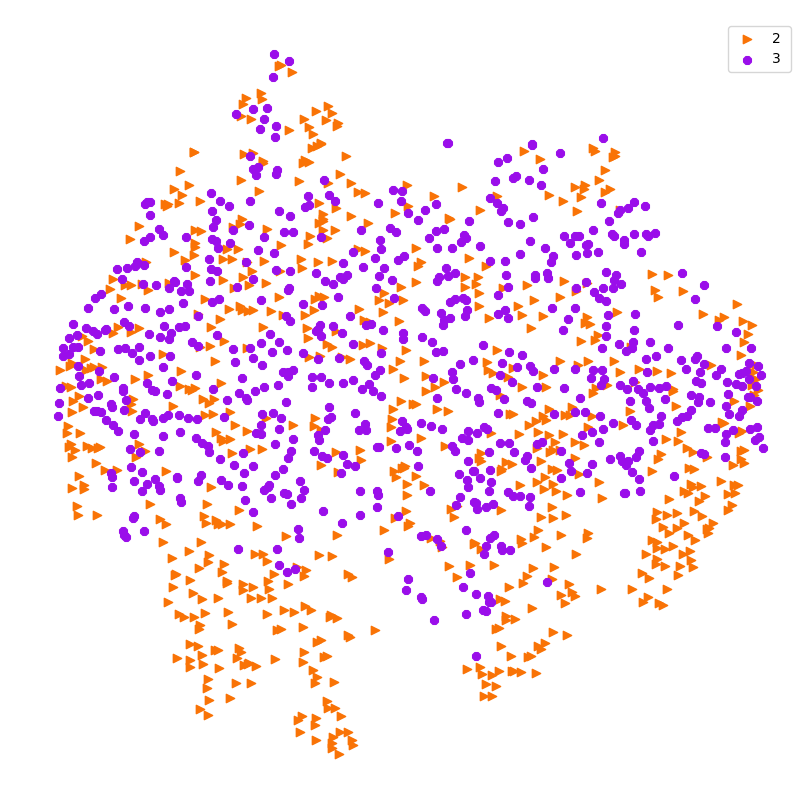} % Reduce the figure size so that it is slightly narrower than the column.
\captionsetup{font=footnotesize}
\caption{} 
\label{fig:sv_str_tsk2}
\end{subfigure}
\begin{subfigure}[b]{.18\linewidth}
\fontsize{7}{9}\selectfont
\includegraphics[width=\textwidth]{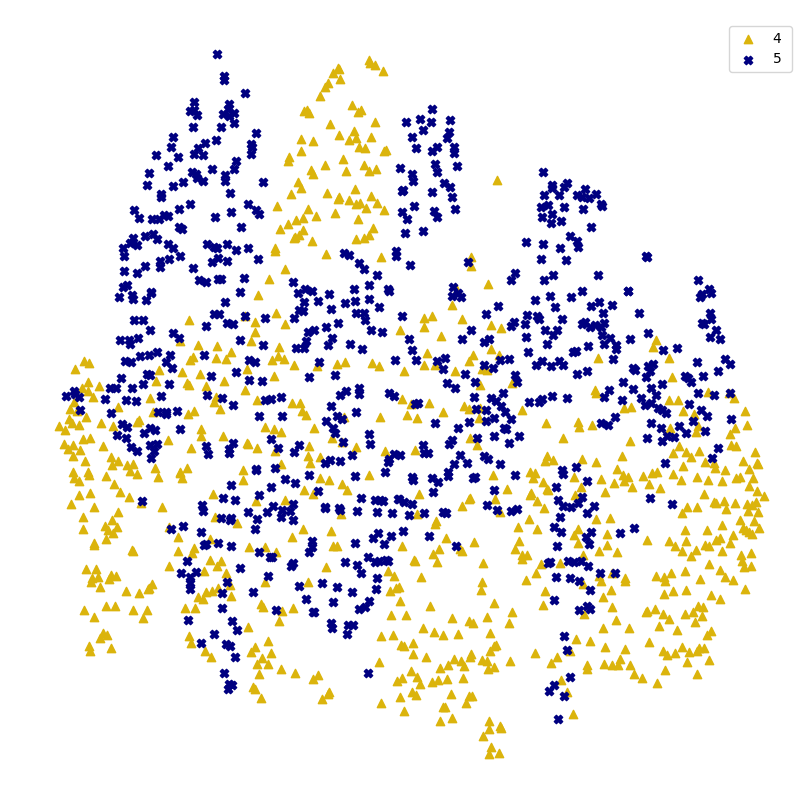} % Reduce the figure size so that it is slightly narrower than the column.
\captionsetup{font=footnotesize}
\caption{} 
\label{fig:sv_str_tsk3}
\end{subfigure}
\begin{subfigure}[b]{.18\linewidth}
\fontsize{7}{9}\selectfont
\includegraphics[width=\textwidth]{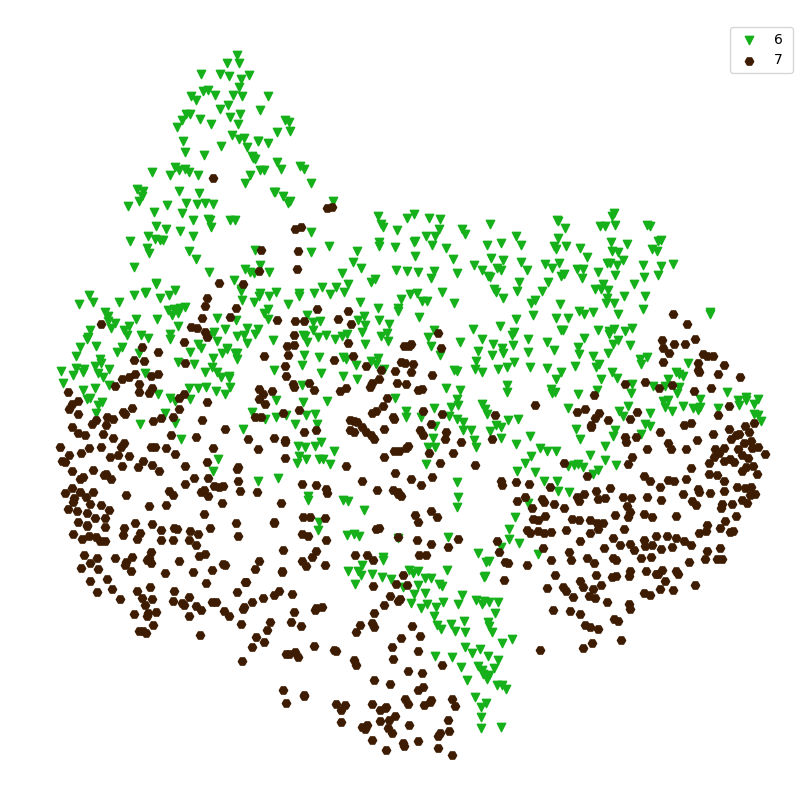} % Reduce the figure size so that it is slightly narrower than the column.
\captionsetup{font=footnotesize}
\caption{} 
\label{fig:sv_str_tsk4}
\end{subfigure}
\begin{subfigure}[b]{.18\linewidth}
\fontsize{7}{9}\selectfont
\includegraphics[width=\textwidth]{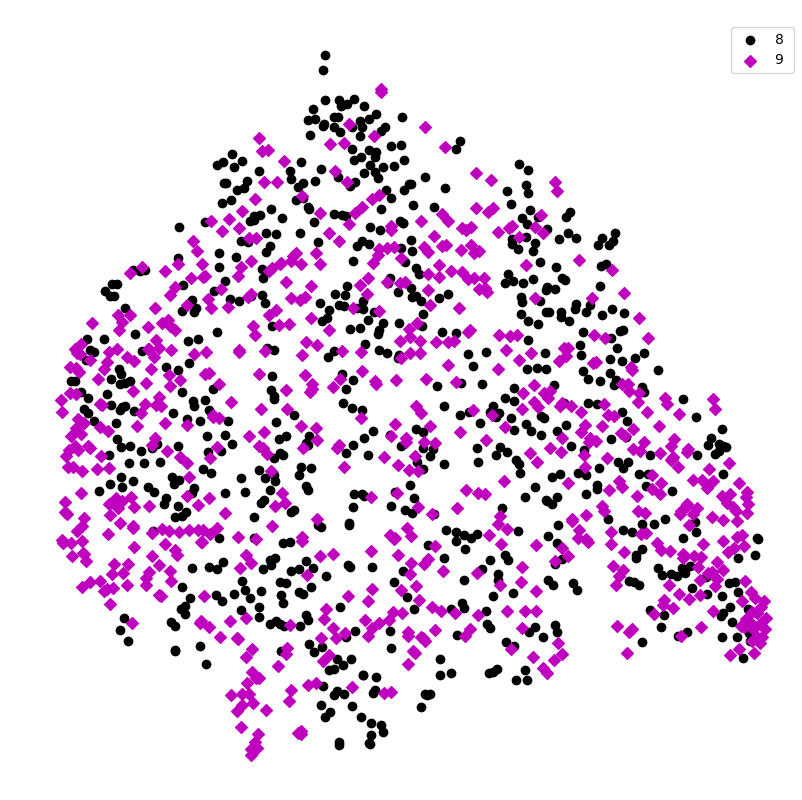} % Reduce the figure size so that it is slightly narrower than the column.
\captionsetup{font=footnotesize}
\caption{} 
\label{fig:sv_str_tsk5}
\end{subfigure}
\captionsetup{font=footnotesize}
\caption{(a)-(e) t-SNE plot of original task data $t_1$ to $t_5$ distribution, (e)-(f) t-SNE plot of generated task data $t_1$ to $t_5$ distribution.} 
\end{figure*}

\section{Memory Efficiency}
\label{AppendixD}
Memory efficiency of various models discussed in section \ref{tab:mem_eff} are calculated as follows:
\vskip 0.1in
\noindent 1. SCALE\cite{yu2023scale}: This model stores 128 samples per class in the storage buffer.  Hence, the memory requirement for SMNIST is,

\noindent $(1280\times28\times28\times4 )$ floating point values $\div 10^6$ $\approx$ 4 MB.
\vskip 0.05in
\noindent Memory requirement for SSVHN data is given by,

\noindent $(1280\times32\times32\times3\times4 )$ floating point values $\div 10^6$ $\approx$ 15.7 MB.
\vskip 0.1in
\noindent 2. KIERA \cite{pratama2021unsupervised}: The number of replay samples are dataset dependent. The memory requirement for SMNIST is given by,

\noindent $(1000\times28\times28\times4 )$ floating point values $\div 10^6$ $\approx$ 3 MB.
\vskip 0.05in
\noindent Memory requirement for SSVHN data is given by,

\noindent $(2300\times32\times32\times3\times4 )$ floating point values $\div 10^6$ $\approx$ 28 MB.
\vskip 0.1in
\noindent 3. UPL-STAM \cite{smith2021unsupervised}: The model stores the centroids in STM and LTM buffers. The total memory requirement is calculated using the following expression \cite{smith2021unsupervised},
\begin{equation}\label{uplmem}
 M = 
\sum_{l=1}^{\Lambda} \rho_l^2 .\Delta + 
\sum_{l=1}^{\Lambda} \rho_l^2 . |C_l|,  \\
 \end{equation}

\noindent where $\rho_l, \Delta, \Lambda, C_l$ refer to patch size, STM capacity, number of layers and set of centroids at layer $l$ respectively.
For more details, please refer to \cite{smith2021unsupervised}. Memory requirement for SMNIST is given by,

\noindent(($8^2\times400$+$13^2\times400$+$20^2\times400$)+($8^2\times1200$+$13^2\times1250$+$20^2\times1600$))$\times4$ floating point values $\div 10^6$ $\approx$ 4.7 MB.
\vskip 0.05in
\noindent Memory requirement for SSVHN is given by,

\noindent(($10^2\times2000$+$14^2\times2000$+$18^2\times2000$)+($10^2\times2600$+$14^2\times2700$+$18^2\times3000$))$\times4$ 
 floating point values $\div 10^6$ $\approx$ 12 MB.
\vskip 0.1in
\noindent 4. UExL: Our proposed model stores the compressed latent space signatures of the task distributions. Hence, the memory requirement is dependent on the latent space dimension. The memory requirement is given by,
\begin{equation}\label{uexlmem}
 M = 
2(dkn_k)+d^2kn_k,\\
 \end{equation}
\noindent where $d$ refers to latent space dimensionality, $k$ is the total number of tasks and $n_k$ is the number of classes per task.
\vskip 0.05in
\noindent Memory requirement for SMNIST is given by,

\noindent($64\times10\times2+64^2\times10) \times4$ floating point values $\div 10^6 \approx 0.17$ MB.
\vskip 0.05in 
\noindent Memory requirement for SSVHN is given by,

\noindent$(128\times10\times2+128^2\times10)\times4$ floating point values $\div 10^6 \approx 0.67$ MB.
